# Supplementary material for: CO-Search: COVID-19 Information Retrieval with Semantic Search, Question Answering, and Abstractive Summarization
Source: arXiv:2006.09595 source file (2020-06-17)
Supplement: Supplementary file 1 [file supplemental.tex]

\section{Supplemental}
